# Supplementary material for: FedCau: A Proactive Stop Policy for Communication and Computation Efficient Federated Learning
Source: arXiv:2204.07773 source file (2024-03-26)
Supplement: Supplementary file 1 [file OldMaterials_Appendix.tex]

%%____________________________________________________________________________
%Then, $R_i  = R_1 + R_2 + R_3 + R_4$ and $R_K = KR_i$ is the total delay with respect to considering solver delay and $K$ is number of iterations running in solver. The optimization problem would be :   
 %\begin{equation}
% g^\star = \underset{\epsilon}{\mathrm{minimize}}  \hspace{1.6mm} \beta \sum_{i=1}^{K}  \hspace{1.6mm}R_i(1-\b1_{\triangle_i < \epsilon_i})+(1-\beta)f(w_{i^\star}), 
 %\end{equation}
% \begin{equation}
%    w_{i+1} = \b1_{\triangle_i > \epsilon_i}(w_i - \alpha_i \nabla_w(f(w_i))) + (1 -\b1_{\triangle_i > \epsilon_i}) w_i ,
%\end{equation}
%%%%%  PLUS ; :::: %%%%%%%
%\subsection{Overall set up }
%In this section, we explain the overall set up for our proposed distributed model. As mentioned before, we consider a centralized distributed set up with a master node and $N$ nodes as workers. We also assume that this network is using a specific channel (like Slotted aloha or CSMA) with a background traffic, $G_B$, as its general variable offered load to which the gradients traffic, $G_O$ would be added. We will consider synchronous and asynchronous approaches for each channel model with particular retransmission policy in the case of an unsuccessful attempt.The goal is to obtain a distribution of maximum delay for this centralized distributed model by utilizing two different algorithms: usual and plus. Finally, we will work on optimizing the obtained maximum delay distribution.       
%\subsection{Our proposed model}
%\begin{remark}
%In our model, we consider that each gradient unit has a constant number of bits ($L$). However, we cannot consider the channel to be constant bit rate (CBR), for the transmission time is not constant. Therefore, for the sake of simplicity, we assume that the gradient offered load has a Poisson distribution with mean $G_O$. As we know, the background traffic has a Poisson distribution. In this case, the total offered load to the channel would have a Poisson distribution with mean $G = G_B + G_O$, because sum of two random variables with Poisson distribution is a random variable with Poisson distribution and its mean is equal to sum of their corresponding means.    
%\end{remark}
%\subsection{ Definitions}
%\subsubsection{Binary Exponential Backoff (BEB) retransmission policy} 
%When a packet transmission fails, a retransmission is scheduled after a random backoff delay which is determined by a specific retransmission policy. If $B_i$ is the $i$th backoff delay in unit of slots, then the $i$th retransmission takes place at the beginning of the $B_i$th available slot after knowing the last transmission is unsuccessful. The delay performance of a random access system depends strongly on the distribution of $B_i$. In our model, we consider binary exponential backoff (BEB) policy in which the backoff delay is uniformly distributed in a binary exponentially expanding range. In other words, the range of backoff delay is doubled every time an unsuccessful retransmission occurs. Let $b$ be the initial backoff range, the $B_i$ is uniformly distributed in $[1, 2^{i-1}b]$.  
 
%\subsubsection{Plus Algorithm}
%In this algorithm, nodes take advantage of the defined backoff time for calculating more units of gradients. Therefore, if a node has an unsuccessful transmission, it would gain extra time (equal to the BEB delay) to update its data which results in a more accurate solution in master node.   
%\subsubsection{Usual Algorithm}
%In this algorithm, despite the plus algorithm master node runs GD with respect to whatever gradient units were calculated during the first time slot for each node. In the other word, nodes are not allowed to use the backoff delay in order to calculate extra units of gradients.

%%%%_________________________________________APPENDIX_____________________________________%%%
 \cleardoublepage 
 \newpage
 
 \appendix

  %\subsection{First Appendix}
  \label{Extra Materials}
%________________________________________________________________________________
%\section{Applications}
%This framework is applicable to 
%\begin{itemize}
%    \item a single solver scenario where there is a cost model for executing iterations of an optimization algorithm and we aim to develop a cost-efficient iterations; and 
 %   \item a general multi-agent scenario where an information exchange is required to take a final decision/inference. 
%\end{itemize}

%\subsection{Autonomous Driving}
%Taking the unfortunate Uber crash example, the cost of running more iterations to find a better solution (e.g., a better solution in transitional optimization problems or a better policy in reinforcement learning) may grow large with time and becomes intolerable (infinity) after a hard deadline, to take \emph{any} decision and to not kill pedestrians. 

%In many other applications as well, the penalty of running more iterations for distributed inference may grow very fast when the network dynamic changes due to high mobility and the decision, even thought to be optimal, becomes obsolete. In that case, we should penalize running more iterations for an inference task.  

%\subsection{Intra-body Sensor Networks}
%Harsh channel environments of intra-body sensor networks and very low-power sensors may severely limit the communication rate. In that case, taking one more iteration may have a huge penalty, whose magnitude may further increase with $k$.  

%\subsection{Edge Computing}
%Here, we may have edge devices with a very limited computational/power capabilities. The cost model can penalize taking more iterations, and our algorithm is a natural fit here. 

%\subsection{Cost-efficient Iterations}
%Consider running an optimization algorithm on a rental server. The current model is that the server charges us linearly in time. In that case, it might be enough to analyze the convergence as a function of the iterations, assuming same cost per iterations. However, our approach may lead to new charging policy that benefits both clients to pay less and the server to make sure less-urgent (more-relaxed) problems will be terminated sooner, leaving more computational resources for more urgent ones at a lower cost. 
%__________________________________________________________________________________________________
\section{Potential Approaches}

\subsection{Approach 2: Penalty Functions}
 Consider a convex and $L$-smooth objective function $f$, the optimization problem is (we start by an unconstrained optimization problem for the sake of simplicity):
\begin{equation}\label{eq: new optimization}
   \underset{w}{\mathrm{minimize}} \hspace{1.6mm} p(f(w),k) \: , 
\end{equation}
where $p(f(w),k): {\mathrm{dom}}~f \times \mathbb{N}\to \mathbb{R}$ is a smooth approximation of $f$ around $w_k$. The idea is to make $f$ sequentially smoother, leading to a faster convergence to an approximate point. An example of $p(f(w),k)$ could be~\cite{duchi2015optimal} 
\begin{equation}
   p(f(w),k) = \mathbb{E}_(f(w_k+\delta)) \:,
\end{equation}
where $\delta$ is a zero-mean Gaussian variable with variance $\sigma_k$. The function $p(f(w),k) $ is equal to $f(w)$ when $\sigma_k$ is near zero for some iterations $k$. The tradeoff here is that for a small $\sigma$, $p(f(w),k) $ may not be very smooth, imposing same complexity on the convergence of iterative algorithm; whereas for a very big $\sigma$, the $f$ may have been to smoothed and we may have altered the local geometry of $f$. In that case, the minimizer of $p(f(w),k) $ may not be close to that of $f(w)$ anymore. Having a smoother function (lower $L$) allows the choice of larger step-sizes (respecting upper-bound of $1/L$ \cite{nesterov2013introductory}) and faster convergence. Therefore, by a proper choice of the step-size parameter, it will be possible to have a faster convergence for the optimization problem.

The next step after obtaining $f_p(w_k)$ is to run GD algorithm for every $f_k (w_k)$, ( we assume $\bP_k$ is differentiable).

Under two extreme situations (infinite$\bJ_1$ and zero $\bP_k$) we are able to recover the usual GD algorithm without any penalty function.The main challenge of this approach is the changes of objective function in every iteration which results in a non-converging solution for the first optimization problem.  
\subsubsection{Challenge}

A challenge here is how to specify the choice of cost model of iterations to iterative smoothening parameter $\delta$ and how to minimize the cost afterward. One potential approach could be similar to the one of the next section where we minimize the cost plus distance of $\delta_k$ to zero, aggregated over $T$ iterations. 

%__________________________________________________________________________________________________
\section{Decision Threshold Updating}
In this section, we put our focus on the Approach 2. First, we discuss about potential technological applications of this method and next, we  present the model and some numerical results.

\subsection{Technological overview}
As it is mentioned in the previous parts, our model is applicable to every situations in which running more iterations will have a huge and expensive cost either in people's health (like Uber crash) or in spending more money/critical resources. Consider the autonomous driving example, it seems that an exponential cost function is valid and can be used as an objective function when it is so expensive for us to have more number of iterations for a very accurate convergence.\\
In order to be more clear on the technological part in some applications, consider low-latency IoT applications which the cost of every single iteration is noticeable and it is critical to have an optimization over number of iterations. For instance, a hard-deadline cost function is like:

\begin{equation}
     c = \begin{cases} \delta, & K < i^\star \\ +\infty, & \text{otherwise}
     \end{cases} ,
 \end{equation}
where $K$ is number of iterations, $i^\star > 0$ is a finite integer and $\delta$ is a very small parameter ($0 <\delta <<1$) is a finite value. \\ %which presents the cost of running the algorithm for each iteration smaller than $i^\star$ . \\
Another important  technological example is "Delay-sensitive IoT" applications in which the cost are not considered as a hard-deadline function; however, it is crucial to minimize the number of iterations in order to reduce delay. For instance, one can consider the cost of iterations, $c_i$ , as a linear function whose slope varies in different applications/situations. \\
Some other technological applications can be channel estimation, inter/intra-body sensor networks in which taking one more iteration may have an expensive penalty. \\
We are still thinking on this problem in order to specify iteration cost, $c_i$, for each particular application. 
\begin{assumption}
In this report, we assume sequence $(c_i)_{i=1,2,\ldots}$ is given and independent of objective function, $f$, decision threshold, $\epsilon$, and $\bw$. 
\end{assumption}

\subsection{Optimization Problem}
In this section, we propose our optimization problem with some numerical results. We assume our objective function, $f$, is convex and $L$-smooth and use gradient descent for obtaining the optimal solution of $f$.  

%\begin{subequations}
%\begin{alignat}{3}
 %& f^\star = \underset{w}{\mathrm{minimize}}\hspace{1.6mm} f(w) \: ,\\
 %\hspace{1.05cm}
 %%\label{eq: const}
 % &{\text{subject to}} \hspace{1.6mm}\triangle_i <\epsilon_i
 %\end{alignat}
 %\end{subequations}
 
\begin{equation}
%\begin{alignat}{3}
 g^\star = \underset{\epsilon_1, \ldots,\epsilon_K}{\mathrm{minimize}}  \hspace{1.6mm} \beta \sum_{i=1}^{K}  \hspace{1.6mm} c_i(1-\b1_{\triangle_i < \epsilon_i})+(1-\beta)f(w_{i^\star}), 
 %\hspace{1.05cm}
 %\label{eq: const}
 %{\text{subject to}}&  &&\hspace{1.6mm} \epsilon_i \le \epsilon_{i+1} ,\hspace{1.6mm}  \forall i
 %\end{alignat}
 \end{equation}
where $c_i$ is the cost for every iteration i, $\epsilon_i$ is the decision threshold at iteration $i$, $i^\star$ is the iteration in which the optimum cumulative iteration cost, $g^\star$, is obtained and $f(w_{i^\star})$ is the value of objective function after $i^\star$ iterations. %The eq. 11b is a natural constraint for descent algorithms, as $\Delta_i$ will be decreased by every iteration. Also, if the observation holds, we need to decide only on one single $\epsilon$ to say when to terminate  the iterations 

In a general case of online optimization when $c_i$ is also unkonwn a priori, and we can have an estimation of that for the next few iterations, we cannot use the threshold policy anymore. To become more specific in solving the optimization problem, we use 
\begin{equation}
    w_{i+1} = \b1_{\triangle_i > \epsilon_i}(w_i - \alpha_i \nabla_w(f(w_i))) + (1 -\b1_{\triangle_i > \epsilon_i}) w_i ,
\end{equation}
where $\alpha_i$ is the step-size for GD method. The first sentence in last equation means that since the decision threshold is not satisfied, the solver should utilize GD method for the optimization problem. While the second sentence reveals that after satisfying the decision threshold at iteration $i^\star$, the value of $w_{i+1}$ will not change. This equation makes sure that the iteration cost are considered just for $i^\star$ number of iterations.   


\section{Analyzing model for different epsilon and iteration cost values}
In this section, we investigate the behaviour of our model for different values of $\epsilon$ and iteration cost $c_i$. We consider a very small $\epsilon = 10^{-5}$, optimal $\epsilon$ with respect to the minimum value of the cost function and a large value, $\epsilon = 1.5$. Then, we take into account three different types of $c_i$ for each value of $\epsilon$ and observe the behaviour of objective function, $f$, and cost function, $g$, according to this set up.      
\subsection{Finding the optimal constant $\epsilon$ for each type of iteration cost}
We consider $w = [w_1 , w_2]^T$, $f(w) = w_1^2 + (w_2-1)^2$ as our objective function and $\beta = 0.5$. Remember the optimization problem
\begin{equation}
 g^\star = \underset{\epsilon_1, ...,\epsilon_K}{\mathrm{minimize}}  \hspace{1.6mm} \beta \sum_{i=1}^{K}  \hspace{1.6mm} c_i(1-\b1_{\triangle_i < \epsilon_i})+(1-\beta)f(w_{i^\star}), 
 \end{equation}
 \begin{equation}
    w_{i+1} = \b1_{\triangle_i > \epsilon_i}(w_i - \alpha_i \nabla_w(f(w_i))) + (1 -\b1_{\triangle_i > \epsilon_i}) w_i ,
\end{equation}
for now, we consider a single threshold and explain how we found the optimal constant $\epsilon$ numerically which results in a smaller cost function for each type of iteration cost. The main idea is to use the exhaustive search for this goal. Therefore, we set the amount of $\epsilon$ to change from $10^{-5}$ to $0.25$ in $K=25000$ steps. Since the constant optimal $\epsilon$ depends on the type and values of $c_i$, we calculated it for every three different types of $c_i$ like:
\begin{align*}
\text{constant cost}: & c_i = 0.0002 \\
\text{linear cost}: & c_i = 0.002i , &  1 \le i \le K  \\
\text{exponential cost}: & c_i = \exp(0.01i) - 1 , & 1 \le i \le K
\end{align*}
The optimal constant $\epsilon$ is obtained as $\epsilon_1 = 0.0142$ for constant cost, $\epsilon_2 = 0.1067$ for linear cost and $\epsilon_3 = 0.2493$ for exponential cost.
%%%%%%%%%%%%%%%%%%%%%%%%%%%%% figures %%%%%%%%%%%%%%%%%%%%%%%
\begin{figure}[t]
 \includegraphics[width=1.1\columnwidth]{Figures/gall.png}
%\captionsetup{justification=centering} 
\centering
  \caption{ Cost function $g$ for constant, linear and exponential iteration cost $c_i$ by three different values of $\epsilon$.
  }%\label{fig: SuperframeStructure}
\end{figure}

\begin{figure}[t]
 \centering
 \includegraphics[width=1.1\columnwidth]{Figures/fall.png} 
%\begin{cente}
  \caption{  objective function $f$ for constant, linear and exponential iteration cost $c_i$ by three different values of $\epsilon$.
  %\end{center}
  }%\label{fig: SuperframeStructure}
\end{figure}
%%%%%%%%%%%%%%%%%%%%%%%%%%%%%%%%%%%%%%%%%%%%%%%%%%%%%%%%%%%%%
\subsection{Cost and Objective function for constant cost}
In this part, we analyze the behaviour of the model by considering a small constant cost for each iteration. The results for cost and objective function are shown in the first subplot of Fig. 1 and Fig. 2. If we take an exact look at the results, it is obtained that the behaviour of the cost function, $g$, is similar for the case of $\epsilon = 10^{-5}$ and optimal $\epsilon_1 = 0.0142$ except for the last iteration in which the cost function is a little smaller for optimal $\epsilon$ case ($g_{\epsilon_{optimal}}^\star = 0.1747$ and $g_{\epsilon = 10^{-5}}^\star = 0.1748$). In the case of having a larger $\epsilon$ ($\epsilon = 1.5$), the algorithm will stop after two iterations and the value of cost function, $g$, will remain constant ($g_{\epsilon = 1.5}^\star = 8.302$). Also, if we look at the first subplot in the Fig. 2. for behaviour of objective function, it is clear that for $\epsilon = 1.5$ the algorithm stops after the second iteration and the terminated objective value is $f_{\epsilon = 1.5} = 16.6$ . However, in the case of optimal and small constant $\epsilon$, the iterations continue and there is no termination in the algorithm, for the threshold $\triangle_i < \epsilon_i$ is not satisfied yet. This means that when the iteration cost $c_i$ are too small, the behaviour of objective function for constant small and optimal $\epsilon$ are similar (by small changes in the large number of iterations).
\subsection{Cost and Objective function for linear iteration cost}
In this part, we consider linear iteration cost and analyze the results in the cost, ($g$), and objective function, ($f$). In the case of $\epsilon = 1.5$, the behaviour of $g$ and $f$ is similar to the previous part and the algorithm terminates after two iterations ($g_{\epsilon = 1.5}^\star = 8.304$ and $f_{\epsilon = 1.5} = 16.6$). However, there are some changes in the case of constant optimal and small $\epsilon$ in this part. As it is shown in the second subplot of Fig. 1, in the case of $\epsilon = 10^{-5} $, $g$ is a decreasing function before the $50^{th}$ iteration and after that, it start increasing. But, for the case of constant optimal $\epsilon$, the value of $g$ remains without change after the $50^{th}$ iteration ($g_{\epsilon_{optimal}}^\star = g_{\epsilon =10^{-5}}^\star = 2.468$ ). On the other hand, the objective functions in the second subplot in Fig. 2, reveal a decreasing function for the case of small $\epsilon$. As a result, the case of constant optimal $\epsilon$ has a better performance in order to find the smaller cost function ($g$) for the linear iteration cost. However, it terminates the algorithm in a point with a larger value of objective function. 
\subsection{Cost and Objective function for exponential iteration cost}
In this part, we choose the iteration cost to be exponential. In the case of $\epsilon = 1.5$, behaviour of $f$ and $g$ is similar to the previous parts, because the algorithm terminates after two iterations like before ($g_{\epsilon = 1.5}^\star = 8.316$ and $f_{\epsilon = 1.5} = 16.6$). If we consider constant small and optimal $\epsilon$, the behaviour of $g$ is the same for 29 iterations. After that, $g$ starts increasing by next iterations in an exponential way, but it remains constant for the case of optimal $\epsilon$ (third subplot in Fig. 1). On the other hand, as it is shown in the third subplot of Fig. 2, $f$ is a decreasing function of iterations for $\epsilon = 10^{-5}$ and it remains constant after 29 iterations for the optimal $\epsilon$. In conclusion, in the case of having an exponential iteration cost, our model shows that the performance of optimal epsilon with respect to minimize the iteration cost function is the best among other kinds of $\epsilon$.    

\newtheorem{thm}{Theorem}
\begin{thm}
The algorithm termination criteria is the same for both constant optimal $\epsilon$ and non-constant (increasing) sequence of $\epsilon$. 
\proof For any set of monotonically increasing $\epsilon_{nc}$, we can always find $\epsilon_c$ such that $t_{nc} = t_c$.  Let $\epsilon_{nc}(t_{nc})$ denote the ${t_{nc}}^{th}$ value of $\epsilon_{nc}$ for which the termination policy is met for the first time. Set $\epsilon_c = \epsilon_{nc}(t_{nc})$. Then prove that $t_c$ would be equal to $t_{nc}$, proving that $g_c = g_{nc}$ for any $t_c$, including $t_{nc}^\star$. This proves that 
$g_{nc}^\star$ $\leq$ $g_c^\star$. Moreover, using a similar proof (starting from any $t_c^\star$ concludes that there is a sequence of $\epsilon_{nc}$ such that $t_{nc}^\star = t_c^\star$ shows that $g_c^\star \leq g_{nc}^\star$. This concludes the proof $g_{nc}^\star = g_c^\star$  
\end{thm}
\begin{remark}
For any $0 \le \beta \le 1$ and $\epsilon$, $g(\epsilon^\star) \le g(\epsilon)$.
\proof First, we consider two extreme cases. \\
Extreme case 1 : $\beta = 0$ \\ Regarding $(11)$, the optimization problem is
\begin{equation}
    g^\star = \underset{\epsilon_1, ...,\epsilon_K}{\mathrm{minimize}}  \hspace{1.6mm} f(w_{i^\star}),
\end{equation}
in which the iteration cost $c_i$ does not matter for the optimization problem and $i^\star$ can be a large number. Therefore, $\epsilon^\star = 0$ which results in finding the $f(w_{i^\star})$ such that $f(w_{i^\star}) = f^\star$. As a result of the convergence of the algorithm, we have $g(\epsilon^\star) \le g(\epsilon)$ , $\forall \epsilon$. \\ \\
Extreme case 2 : $\beta = 1$ \\
In this case the optimization problem is
\begin{equation}
 g^\star = \underset{\epsilon_1, ...,\epsilon_K}{\mathrm{minimize}}  \hspace{1.6mm} \sum_{i=1}^{K}  \hspace{1.6mm} c_i(1-\b1_{\triangle_i < \epsilon_i}), 
 \end{equation}
in which the value of $f(w_{i^\star})$ does not affect the iteration cost function, $g$. So, the only focus of the optimization problem is on the iteration cost $c_i$ and since $c_i > 0$, it is crucial to have the minimum value of iteration cost which is gained when the algorithm stops after just one iteration. In this case, $g(\epsilon^\star) = g^\star = c_1$ and $\epsilon^\star = +\infty$. Therefore, $g(\epsilon^\star) \le g(\epsilon)$, $\forall \epsilon$. \\
As we showed, the statement is applied to the two extreme cases. In general when we have $0 < \beta < 1 $ and as mentioned in the definition of the main optimization problem, $g(\epsilon^\star)$ is the optimal solution for $(11)$. Therefore, for every $0 < \beta < 1 $, $\exists \epsilon^\star$ which $\epsilon^\star$ is the element for finding the optimal solution of minimization problem $(11)$. Therefore, by definition of $(11)$, $g^\star = g(\epsilon^\star)$ and $g(\epsilon^\star) \le g(\epsilon)$, $\forall \epsilon$ and $\forall \beta$.
\end{remark}
\section{Causal Algorithm}
In this part, we put our focus on developing a causal algorithm for optimization problem $(11)$. In practice, $(11)$ is not a causal algorithm, for we assumed that the values of $\bw$ and $f(w)$ and all the $c_i$ are available. However, in the real world, we do not have access to these values in order to find the optimal $\epsilon^\star$. In this situation, it is crucial to propose a causal method to predict the values of $\bw$ and $f(w)$ for next iterations. For the sake of simplicity, we still consider that $c_i$ is a fixed given sequence. %As our optimization algorithm is GD, we are able to use the available defined upper bounds on $f(w)$ for prediction.

\subsection{Causal algorithm with adaptive $\epsilon$}
In this part we propose a simple causal algorithm which depends on the derivative of $g$ function. As we  know, in descent methods for convex functions, the value of objective function would decrease when the iterations pass. Therefore, we can always say that the $g$ function will have just one minimum value which is accessible by considering the sign of difference of two consecutive $g$ such that :
\begin{equation}
    g_i - g_{i-1} = \beta c_i + (1 - \beta)(f(w_i) - f(w_{i-1}))
\end{equation}
after each iteration $i$ (the derivative sign). In the beginning, the solver sets $\epsilon = +\infty$ in order to make sure that the iteration would continue. If the mentioned sign is negative, it means that the $g$ function is decreasing and we have not found the minimum yet. As soon as the sign turns positive, the algorithm would terminate by setting the value of $\epsilon = 0$ and then solver reports the corresponding values for $g$ and $f$. This approach requires one more iteration than the non-causal algorithm which satisfies $(30)$ and
\begin{subequations}
\begin{alignat}{3}
 &  f(w_{i_{nc}^\star}) > f(w_{i_{c}^\star}) \: ,\\
 \hspace{1.05cm}
 %%\label{eq: const}
  & g_{i_{c}^\star} > g_{i_{nc}^\star}. \\ 
 \end{alignat}
 \end{subequations}
The results of this algorithm are shown in Fig. 3-5.
%%%%%%%%%%%%%%%%%%%%%%%%%%%%% figures %%%%%%%%%%%%%%%%%%%%%%%

\begin{figure}
 \includegraphics[width=1.1\columnwidth]{Figures/s1 constantc.png}
%\captionsetup{justification=centering} 
\centering
  \caption{ $g$, stopping point and ¤$f$ in non-causal and causal algorithm with adaptive $\epsilon$ for constant iteration cost $c_i = 0.0002$ .
  }%\label{fig: SuperframeStructure}
\end{figure}
\begin{figure}[t]
 \includegraphics[width=1.1\columnwidth]{Figures/s1 linearc.png}
%\captionsetup{justification=centering} 
\centering
  \caption{ $g$, stopping point and ¤$f$ in non-causal and causal algorithm with adaptive $\epsilon$ for linear iteration cost.
  }%\label{fig: SuperframeStructure}
\end{figure}
\begin{figure}
 \includegraphics[width=1.1\columnwidth]{Figures/s1 expc.png}
%\captionsetup{justification=centering} 
\centering
  \caption{ $g$, stopping point and ¤$f$ in non-causal and causal algorithm with adaptive $\epsilon$ for exponential iteration cost .
  }%\label{fig: SuperframeStructure}
\end{figure}
%__________________________________________________________________________________________________
\subsection{Causal Approximation with Upper Bound For Convex and $L$-smooth function }

We consider a convex and $L$-smooth objective function $f$. So, the well-known upper bound is
\begin{equation}
    %\|f(w_i) - f^\star\| \le \frac {\| w_0 - w^\star \|^2 }{2i\alpha}
    f(w_i) - f^\star \le \frac {2L\gamma_0 \| w_0 - w^\star \|^2 }{(i+4)}
\end{equation}
where $\gamma_i = f(w_i) - f*$.
\begin{assumption}
We assume that the value $f^\star = 0$.
\end{assumption}
\begin{assumption}
$\forall x,y \in \chi, \|x-y\|_2^2 \le R^2 , R > 0 $.
\end{assumption}
By these two assumptions, we can rewrite $(17)$ as
\begin{equation}
    f(w_i) \le \frac {2Lf(w_0)R^2 }{(i+4)}
\end{equation}
%\begin{equation}
 %   \|f(w_i)\| \le \frac {\| w_0 - w^\star \|^2 }{2i\alpha}.
%\end{equation}
Therefore, we use the upper bound $(18)$ as a prediction for the value of objective function $f$ at next iterations in our algorithm, ($\Tilde{f}(w_i)$). If we consider $g_{nc}$ and $g_{c}$ as the iteration cost functions for $f$ and $\Tilde{f}$ and also $i_{nc}^\star$ and $i_{c}^\star$ as stopping iteration point for them, we have
\begin{equation}
  g_{nc}^\star = \underset{\epsilon}{\mathrm{minimize}}  \hspace{1.6mm} \beta \sum_{i=1}^{K}  \hspace{1.6mm} c_i(1-\b1_{\triangle_i < \epsilon})+(1-\beta)f(w_{i_{nc}^\star}),  
\end{equation}
\begin{equation}
  g_{c}^\star = \underset{\epsilon}{\mathrm{minimize}}  \hspace{1.6mm} \beta \sum_{i=1}^{K}  \hspace{1.6mm} c_i(1-\b1_{\triangle_i < \epsilon})+(1-\beta)\Tilde{f}(w_{i_{c}^\star}).  
\end{equation}
The elements for optimal solutions of $(19)$ and $(20)$ are $\epsilon_{nc}^\star$ and $\epsilon_{c}^\star$ such that
\begin{equation}
  \epsilon_{nc}^\star \in \underset{\epsilon}{\mathrm{arg min}}  \hspace{1.6mm} \beta \sum_{i=1}^{K}  \hspace{1.6mm} c_i(1-\b1_{\triangle_i < \epsilon})+(1-\beta)f(w_{i_{nc}^\star}),  
\end{equation}
and
\begin{equation}
  \epsilon_{c}^\star \in \underset{\epsilon}{\mathrm{arg min}}  \hspace{1.6mm} \beta \sum_{i=1}^{K}  \hspace{1.6mm} c_i(1-\b1_{\triangle_i < \epsilon})+(1-\beta)\Tilde{f}(w_{i_{c}^\star}).  
\end{equation}
As $\Tilde{f}$ is an upper bound on $f$, it overestimates the value of objective function at each iteration. It means that $g_{nc}^\star \le g_{c}^\star$; therefore, we can say that $\epsilon_{c}^\star \le \epsilon_{nc}^\star$ and $i_{nc}^\star \le i_{c}^\star$.
\begin{remark}
The prediction of $f(w)$ becomes more accurate by using an adaptive upper bound instead of a fixed one which results in converging to the actual optimal solution.
\begin{equation}
  g(\epsilon , j) = \beta \sum_{i=1}^{K}  \hspace{1.6mm} c_i(1-\b1_{\triangle_i < \epsilon_i})+(1-\beta)\Tilde{f}(w_{i^\star})  
\end{equation}
where $j$ is the iteration in which upper bound would be updated.
\end{remark}
\subsection{Sequential Causal Approximation For Convex and $L$-smooth function }
In this part we propose the sequential causal approximation method in order to improve the upper bound used for approximation the objective function in the next iterations. Consider
\begin{equation}
   \epsilon_{cl(m)}^\star \in \underset{\epsilon}{\mathrm{arg min}}  \hspace{1.6mm} \beta \sum_{i=1}^{K}  \hspace{1.6mm} c_i(1-\b1_{\triangle_i < \epsilon})+(1-\beta)\Tilde{f}_K(m) 
\end{equation}
where $ \Tilde{f}_{K(m)} = (f_1, f_2, ..., f_m, f_j) $ in which $f_i,\hspace{1.2mm} i = 1, ..., m$ are the values of objective function $f$ after $m$ iterations and $f_j$ is defined as
\begin{equation}
    f_j := \frac {2Lf_mR^2 }{(j-m+4)}, \hspace{1.8mm} j = m+1, ..., K
\end{equation}
where $f_j$ is approximation for the value of objective function for next $K-m$ iterations. So, we can use $(25)$ for calculating the iteration cost function $g$ by running the GD algorithm to find the optimal solution. A brief this approach is shown in the following chart.
\\ \newline
%% Flowchart for sequential causal approximation%%%%%
\begin{figure}{}
   \centering
   \begin{subfigure}[b]{0.3\textwidth}
         \centering
  %  \includegraphics{}
\tikzstyle{startstop} = [rectangle, rounded corners, minimum width=3cm, minimum height=1cm,text centered, draw=black, fill=white!30]
\tikzstyle{io} = [trapezium, trapezium left angle=70, trapezium right angle=110, minimum width=3cm, minimum height=1cm, text centered, draw=black, fill=white!30]
\tikzstyle{process} = [rectangle, minimum width=3cm, minimum height=1cm, text centered, draw=black, fill=white!30]
\tikzstyle{decision} = [diamond, minimum width=3cm, minimum height=1cm, text centered, draw=black, fill=white!30]
\tikzstyle{arrow} = [thick,->,>=stealth]
\begin{tikzpicture}[node distance=2cm]
%\node (start) [startstop] {Start};
\node (pro1) [process, xshift=4cm] {Iteration $i\Leftarrow i+1$};
\node (pro2) [process, below of=pro1] {Solve $(25)$};
\node (pro3) [process, below of=pro2] {Run GD with new $\epsilon_{c}^\star(i)$};
\node (dec1) [decision, left of=pro3, xshift=-2cm] {$i < K $};
\node (pro4) [process, below of= dec1] {Report $\epsilon_{cl(m)}^\star$ };
%\draw [arrow] (start) -| (pro1);
\draw [arrow] (pro1) -- (pro2);
\draw [arrow] (pro2) -- (pro3);
\draw [arrow] (pro3) -- (dec1);
\draw [arrow] (dec1) |- node[anchor=east] {yes} (pro1);
\draw [arrow] (dec1) -- node[anchor=east] {no} (pro4);
\end{tikzpicture}
\caption{1 Sequential Causal Approximation for  convex and $L$-smooth objective function}
    \label{fig:chart}
    \end{subfigure}
     \hfill
     \begin{subfigure}[b]{0.3\textwidth}
         \centering
         \tikzstyle{startstop} = [rectangle, rounded corners, minimum width=3cm, minimum height=1cm,text centered, draw=black, fill=white!30]
\tikzstyle{io} = [trapezium, trapezium left angle=70, trapezium right angle=110, minimum width=3cm, minimum height=1cm, text centered, draw=black, fill=white!30]
\tikzstyle{process} = [rectangle, minimum width=3cm, minimum height=1cm, text centered, draw=black, fill=white!30]
\tikzstyle{decision} = [diamond, minimum width=3cm, minimum height=1cm, text centered, draw=black, fill=white!30]
\tikzstyle{arrow} = [thick,->,>=stealth]
\begin{tikzpicture}[node distance=2cm]
\node (start) [startstop] {Solve $(25)$ for $m = 0$};
\node (pro1) [process, below of=start, xshift=4cm] {Iteration $i\Leftarrow i+1$};
\node (pro2) [process, below of=pro1] {Run GD with $\epsilon_{c}^\star(0)$};
\node (dec1) [decision, left of=pro2, xshift=-2cm] {$i < K $};
\node (pro3) [process, below of=dec1] {Report $\epsilon_{c}^\star$ };
\draw [arrow] (start) -| (pro1);
\draw [arrow] (pro1) -- (pro2);
\draw [arrow] (pro2) -- (dec1);
\draw [arrow] (dec1) |- node[anchor=east] {yes} (pro1);
\draw [arrow] (dec1) -- node[anchor=east] {no} (pro3);
\end{tikzpicture}
%\caption{2 Sequential Causal Approximation for  convex and $L$-smooth objective function}
\caption{}
   \end{subfigure}
   \caption{test graph}
\end{figure}
%%______________________________________________________________%%%%%
\\ \newline
\subsubsection{Fixed Causal Approximation}
In order to have a fixed causal approximation, we should set the value of $m$ in $(25)$ to zero; so, we achieve the main upper bound result mentioned in $(18)$. This is a particular case in which we obtain the general upper bound for convex and $L$-smooth functions. The next chart is a brief explanation of this case.
\\ \newline
%%%%%%%%%%%%%%%%%%%_____________________________________________%%%%%%
\tikzstyle{startstop} = [rectangle, rounded corners, minimum width=3cm, minimum height=1cm,text centered, draw=black, fill=white!30]
\tikzstyle{io} = [trapezium, trapezium left angle=70, trapezium right angle=110, minimum width=3cm, minimum height=1cm, text centered, draw=black, fill=white!30]
\tikzstyle{process} = [rectangle, minimum width=3cm, minimum height=1cm, text centered, draw=black, fill=white!30]
\tikzstyle{decision} = [diamond, minimum width=3cm, minimum height=1cm, text centered, draw=black, fill=white!30]
\tikzstyle{arrow} = [thick,->,>=stealth]
\begin{tikzpicture}[node distance=2cm]
\node (start) [startstop] {Solve $(25)$ for $m = 0$};
\node (pro1) [process, below of=start, xshift=4cm] {Iteration $i\Leftarrow i+1$};
\node (pro2) [process, below of=pro1] {Run GD with $\epsilon_{c}^\star(0)$};
\node (dec1) [decision, left of=pro2, xshift=-2cm] {$i < K $};
\node (pro3) [process, below of=dec1] {Report $\epsilon_{c}^\star$ };
\draw [arrow] (start) -| (pro1);
\draw [arrow] (pro1) -- (pro2);
\draw [arrow] (pro2) -- (dec1);
\draw [arrow] (dec1) |- node[anchor=east] {yes} (pro1);
\draw [arrow] (dec1) -- node[anchor=east] {no} (pro3);
\end{tikzpicture}

%%%%%%___________________________________________________%%%%%
\begin{lemma}
If $i_c^\star$ and $i_{nc}^\star$ are the iterations at which the causal and non-causal algorithms terminate, then $i_{nc}^\star \le i_c^\star$.
\proof As we showed in $Remark 1$, $g(\epsilon_{nc}^\star) \le g(\epsilon), 0 \le \beta \le 1, \forall \epsilon$. Also, as we use the upper bound of objective function as an causal approximation, then the causal iteration cost function, $g_{c}(\epsilon)$, would be an upper bound for the non-causal iteration cost function, $g_{nc}(\epsilon)$, ($g_{nc}(\epsilon) \le g_{c}(\epsilon) $ ). Therefore, by combination of $Remark 1$ and this upper bound, we have $g(\epsilon_{nc}^\star) \le g_{nc}(\epsilon) \le g_{c}(\epsilon), \forall \epsilon $, then
\begin{equation}
   g(\epsilon_{nc}^\star) \le g(\epsilon_{c}^\star). \\  
\end{equation}
  We assume that $i_{c}^\star < i_{nc}^\star$. By calculating the difference of non-causal and causal iteration cost functions, $g(\epsilon_{nc}^\star) - g(\epsilon_{c}^\star) = g_{nc}^\star - g_{c}^\star$, we have (according to $(19)$ and $(20)$)
  \begin{equation}
      g_{nc}^\star - g_{c}^\star = \beta \sum_{i=1}^{i_{nc}^\star} c_i+(1-\beta)f(w_{i_{nc}^\star}) - \beta \sum_{i=1}^{i_c^\star} c_i-(1-\beta)\Tilde{f}(w_{i_c^\star}). \\
  \end{equation}
  After simplification, the $(27)$ would be rewritten as
  \begin{equation}
      g_{nc}^\star - g_{c}^\star = \beta \sum_{i=i_c^\star + 1}^{i_{nc}^\star}c_i + (1-\beta)(f(w_{i_{nc}^\star}) -\Tilde{f}(w_{i_c^\star})). \\
  \end{equation}
  According to $26$, we have $g_{nc}^\star - g_{c}^\star \le 0 $, so
  \begin{equation}
     \beta \sum_{i=i_c^\star + 1}^{i_{nc}^\star}c_i + (1-\beta)(f(w_{i_{nc}^\star}) -\Tilde{f}(w_{i_c^\star})) \le 0, \forall \beta. \\
  \end{equation}
  As we assumed $i_{c}^\star < i_{nc}^\star$ which results in $\sum_{i=i_c^\star + 1}^{i_{nc}^\star}c_i > 0$. Also, as $\Tilde{f}(w)$ is an upper bound for $f(w), \forall w $, the second term in $(29)$ is a non-positive value ($f(w_{i_{nc}^\star}) -\Tilde{f}(w_{i_c^\star}) \le 0$). Therefore, by $(29)$, the summation of these two terms by considering the value of $\beta$ should be non-positive for every $ 0 \le \beta \le 1$. However, by considering $\beta = 1$, the second term in $(29)$ will be eliminated from the equation; so, the first term just remains which is a positive value. In this point, we reach a contradiction, for it does not satisfy the $(29)$. Therefore, it results that the assumption of $i_{c}^\star < i_{nc}^\star$ is not true, so that
  \begin{equation}
      i_{nc}^\star \le i_c^\star
  \end{equation}
\end{lemma}
\begin{remark}
In gradient descent method, if $f$ is a convex function and $i > j$ then $||f(w_i) - f(w_{i-1})|| < || f(w_j) - f(w_{j-1})|| $.
\end{remark}
\begin{lemma}
$\epsilon_{c}^\star \le \epsilon_{nc}^\star$ if and only if $i_{nc}^\star \le i_c^\star$.
\proof
 By the definition of $i_{nc}^\star$ and $i_c^\star$ we have
\begin{equation}
  i_{nc}^\star = \min({i}) \hspace{1.6mm} \text{such that} \hspace{1.6mm}{ ||f(w_i) - f(w_{i-1})|| < \epsilon_{nc}^\star}, 
\end{equation}
\begin{equation}
  i_c^\star = min ({i}) \hspace{1.6mm} \text{such that} \hspace{1.6mm} ||f(w_i) - f(w_{i-1})|| < \epsilon_{c}^\star.
\end{equation}
First, we assume that $\epsilon_{c}^\star \le \epsilon_{nc}^\star$, we show that $i_{nc}^\star \le i_c^\star$. As mentioned in $(31)$ and $(32)$, if $\epsilon_{c}^\star \le \epsilon_{nc}^\star$, then $||f(w_{i_{c}^\star}) -f(w_{i_{c}^\star-1})|| \le ||f(w_{i_{nc}^\star}) -f(w_{i_{nc}^\star-1})|| $. According to remark2, we can conclude that $i_{nc}^\star \le i_c^\star$.\\
Second, we consider the reverse part of the statement such that if $i_{nc}^\star \le i_c^\star$, then $\epsilon_{c}^\star \le \epsilon_{nc}^\star$. We assume that $\epsilon_{c}^\star > \epsilon_{nc}^\star$, we have $||f(w_{i_{c}^\star}) -f(w_{i_{c}^\star-1})|| < \epsilon_{c}^\star$ and $||f(w_{i_{nc}^\star}) -f(w_{i_{nc}^\star-1})|| < \epsilon_{nc}^\star$; so, by the remark2 it results that $i_{nc}^\star > i_c^\star$ which is in the contradiction of our statement. It means that the assumption of $\epsilon_{c}^\star > \epsilon_{nc}^\star$ is not true and it results in $\epsilon_{c}^\star \le \epsilon_{nc}^\star$.
\end{lemma}

%%%%%%%%%%%%%%%%%%%%%%%%%%%%%%%%%%%%%%%%%%%%%%%%%%%%%%%%%%%%%
%\subsection{Numerical results}

 %%%% _______NOTICE_______%%%%%%
 % Add the preposition of Tc = Tnc + k , ......
%%%%%%___________________________________________________%%%%%
\subsection{Causal Approximation with Upper Bound For $\mu$-Strongly Convex and $L$-smooth function }
In this part we restrict the objective function to be $\mu$-strongly convex and $L$-smooth. Therefore, the upper bound needed for our causal problem is
\begin{equation}
\| w_i - w^\star \|_2^2 \le (1-\frac{2\alpha \mu L}{L + \mu})^i  \| w_0 - w^\star \|^2,
   % f(w_i) - f^\star \le \frac {2L\gamma_0 \| w_0 - w^\star \|^2 }{(i+4)}
\end{equation}
where $ 0 < \alpha < \frac{2}{L + \mu}$ is the step size for the GD method. If we consider$ \alpha = \frac{2}{L + \mu}$, then  
\begin{equation}
    f(w_i) - f^\star \le \frac{L}{2} (\frac {\kappa -1 }{\kappa + 1})^{2i} \| w_0 - w^\star \|_2^2,
\end{equation}
where $\kappa = \frac{L}{\mu}$ is the condition number.


\subsection{Sequential Causal Approximation For $\mu$-Strongly Convex and $L$-smooth function }
We can propose a sequential causal approximation for $\mu$-strongly convex and $L$-smooth objective function like we did for convex functions. However, this approximation here is not so much better than the actual upper bound, for $ 0 < \frac {\kappa -1 }{\kappa + 1} < 1$ which there is no big improvement if we change power $i$ to $j - m$. 
%\\ (We are still working on the causal approximation.)
%(We are still working on theorem 2 and theorem 3.)
%%%%------------- Application of paper ------------------------%
%\section{Distributed Optimization Considering solver delay}
%In this section, we bring a concrete example for distributed optimization by taking into account the required time for each iteration in GD solver. We consider there are $k$ workers and a master node in the decentralized GD method. Our optimization problem will be:
%\begin{equation}
   % f^\star = {\mathrm{minimize}}  \hspace{1.6mm} \sum_{j=1}^{k}  %\hspace{1.6mm} f_j
%\end{equation}
%\begin{equation}
%\begin{alignat}{3}
%  g^\star = \underset{\epsilon_1, ...,\epsilon_T}{\mathrm{minimize}}  \hspace{1.6mm} \beta \sum_{i=1}^{T}  \hspace{1.6mm} R_{it}(1-\b1_{\triangle_i < \epsilon_i})+(1-\beta)f(w_{i^\star}),
  % \end{equation}
%\begin{equation}
 %  R_{it}= R_1 + kR_2 + R_3 + R_4  
%\end{equation}
%\hspace{1.05cm}
%\end{alignat}
 %\begin{equation}
  %  w_{i+1}^j = \b1_{\triangle_i > \epsilon_i}(w_i^j - \alpha_i \nabla_w(f_j(w_i^j))) + (1 -\b1_{\triangle_i > \epsilon_i}) w_i^j ,  
%\end{equation}
% &{\text{subject to}} \hspace{1.6mm}\triangle_i <\epsilon_i
%where $R_1$ is time required for broadcasting each $w_i$ by master node, $R_2$ is the time needed for computing $\nabla_w(f_j(w_i^j))$ in every worker $j$, $R_3$ is the required time for broadcasting $\nabla_w(f_j(w_i^j))$ to master node and $R_4$ is the computation time in master node.
In this section, we show some numerical results of the causal algorithm
we proposed in previous parts. Like  part $IV$, we consider three types of iteration cost sequences; constant, linear and exponential. Our approach for the causal algorithm is that we approximate a set of $K$ values for objective function $f_0,...,f_K$ during each iteration $i$ such that
\begin{equation}
    f_0,...,f_K = f_0, f_1,...,f_i, \hat {f}_{i+1},...,\hat{f}_j,\Tilde{f}_{j+1},...,\Tilde{f}_K
\end{equation}
where $\hat{f}_{k} = min ({f_i, \Tilde{f}_k})$, $i < k \le j$, which means that in the first $i$ iterations, we should use the true values of objective function ($f_1,...,f_i$), and for other values, we consider the minimum between upper bound estimation and the last true value of $f$. After that, we calculate the minimum value of cost function $g$ and find the corresponding value of $\epsilon$ for it. The results of the causal and non-causal approach are shown in Fig. 6-11. As we see in Fig.7, Fig.9 and Fig.11, the $lemma1$ is not completely true for some iterations. In the following paragraphs, we investigate if the $(29)$ is satisfied for those parts of irregularities. \\ 
\subsubsection{constant $c_i = 0.0002 $}
By a careful look at Fig. 6-7, we recognize there is irregularities from iteration $62$ till $194$ which reveal that $i_c^\star \le i_{nc}^\star$ interpreted as early stopping between these iterations. By considering $i_c^\star = 62$ and $i_{nc}^\star = 194$, $f(w_{i_{c}^\star}) = 0.00738$, $f(w_{i_{nc}^\star}) = 1.5306$ and $\beta = 0.6$, the value of the left side of $(29)$ for this part is $-0.593$ which satisfies the inequality. However, $\epsilon_{c} = 0.0631$ which is greater than $\epsilon_{nc} = 0.00031$. 
\subsubsection{linear $c_i = 0.002i $}
 Fig. 8-9 also show some irregularities from iteration $4$ till $65$ which reveal that $i_c^\star \le i_{nc}^\star$ and interpreted as early stopping between these iterations. By considering $i_c^\star = 4$ and $i_{nc}^\star = 65$, $f(w_{i_{c}^\star}) = 15.9452$, $f(w_{i_{nc}^\star}) = 1.3558$ and $\beta = 0.3 $, the value of the left side of $(29)$ for this part is $-8.93$ which satisfies the inequality. However, $\epsilon_{c} = 0.6575$ which is greater than $\epsilon_{nc} = 0.0559$. 
\subsubsection{exponential $c_i $}
 For this part, like two previous parts,  there are some irregularities from iteration $16$ till $95$ which reveal that $i_c^\star \le i_{nc}^\star$ and interpreted as early stopping between these iterations. By considering $i_c^\star = 16$ and $i_{nc}^\star = 95$, $f(w_{i_{c}^\star}) = 9.8187$, $f(w_{i_{nc}^\star}) = 0.4034$ and $\beta = 0.01 $, the value of the left side of $(29)$ for this part is $-8.7$ which satisfies the inequality. However, $\epsilon_{c} = 0.0443$ which is greater than $\epsilon_{nc} = 0.0167$. 

%%%%%%%%%%%%%%%%%%%%%%%%%%%%% figures %%%%%%%%%%%%%%%%%%%%%%%
\begin{figure}
 \includegraphics[width=1.1\columnwidth]{Figures/c0.0002.png}
%\captionsetup{justification=centering} 
\centering
  \caption{ causal and non-causal results of cost function $g$, stopping point, difference of $\epsilon_{c}$ and $\epsilon_{nc}$, objective function $f$ for constant iteration cost $c_i = 0.0002$ .
  }%\label{fig: SuperframeStructure}
\end{figure}
\begin{figure}
 \includegraphics[width=1.1\columnwidth]{Figures/gs c0.0002.png}
%\captionsetup{justification=centering} 
\centering
  \caption{ $g$ function for three different stopping point in causal algorithm for constant iteration cost $c_i = 0.0002$ .
  }%\label{fig: SuperframeStructure}
\end{figure}
\begin{figure}[t]
 \includegraphics[width=1.1\columnwidth]{Figures/linear c.png}
%\captionsetup{justification=centering} 
\centering
  \caption{ causal and non-causal results of cost function $g$, stopping point, difference of $\epsilon_{c}$ and $\epsilon_{nc}$, objective function $f$ for linear iteration cost.
  }%\label{fig: SuperframeStructure}
\end{figure}
\begin{figure}
 \includegraphics[width=1.1\columnwidth]{Figures/gs linear c.png}
%\captionsetup{justification=centering} 
\centering
  \caption{ $g$ function for three different stopping point in causal algorithm for linear iteration cost .
  }%\label{fig: SuperframeStructure}
\end{figure}
\begin{figure}[t]
 \includegraphics[width=1.1\columnwidth]{Figures/expc.png}
%\captionsetup{justification=centering} 
\centering
  \caption{ causal and non-causal results of cost function $g$, stopping point, difference of $\epsilon_{c}$ and $\epsilon_{nc}$, objective function $f$ for $exponential$ iteration cost.
  }%\label{fig: SuperframeStructure}
\end{figure}
\begin{figure}
 \includegraphics[width=1.1\columnwidth]{Figures/gs expc.png}
%\captionsetup{justification=centering} 
\centering
  \caption{ $g$ function for three different stopping point in causal algorithm for $exponential$ iteration cost .
  }%\label{fig: SuperframeStructure}
\end{figure}
